# Supplementary material for: CutClaw: Agentic Hours-Long Video Editing via Music Synchronization
Source: arXiv:2603.29664 source file (2026-03-31)
Supplement: Supplementary file 1 [file 06_appendix.tex]

% =================================================================
% 附录开始：切换单栏，优化大图展示
% =================================================================
% \onecolumn

% 这一行是为了防止第一页标题被异常挤到下一页（强行增加本页有效高度）
\enlargethispage{5cm} 
\section{Prompt of VideoCuts}

% =================================================================
% 第一部分：Bottom-Up Multimodal Footage Deconstruction
% =================================================================
\subsection{Prompt for Bottom-Up Multimodal Footage Deconstruction}
% \vspace{-0.5cm}
% 【第1张图】与标题在同一页
% 注意：这里限制高度为 0.75\textheight，留出头部空间给标题
\begin{figure}[H]
    \centering
    \includegraphics[width=\textwidth, height=\textheight, keepaspectratio]{vis/fig/Prompt_apx/Shot_parsing.pdf}
\end{figure}
\onecolumn

% 【第2张图】独占一页
\clearpage
\begin{figure}[H]
    \centering
    % 注意：独占页可以更大，设为 0.95\textheight
    \includegraphics[width=0.95\textwidth, height=0.95\textheight, keepaspectratio]{vis/fig/Prompt_apx/Scene_agg.pdf}
\end{figure}

% 【第3张图】独占一页
\clearpage
\begin{figure}[H]
    \centering
    \includegraphics[width=0.95\textwidth, height=0.95\textheight, keepaspectratio]{vis/fig/Prompt_apx/Audio_stru.pdf}
\end{figure}

% 【第4张图】独占一页
\clearpage
\begin{figure}[H]
    \centering
    \includegraphics[width=0.95\textwidth, height=0.95\textheight, keepaspectratio]{vis/fig/Prompt_apx/Audio_key.pdf}
\end{figure}

% =================================================================
% 第二部分：Playwriter
% =================================================================
\clearpage % 强制换页开始新的一节
\enlargethispage{3cm} % 再次确保标题和图在一起

\subsection{Prompt for Playwriter}

% 【第1张图】与标题在同一页 (height=0.75)
\begin{figure}[H]
    \centering
    \includegraphics[width=0.95\textwidth, height=0.95\textheight, keepaspectratio]{vis/fig/Prompt_apx/Pro_gen.pdf}
\end{figure}

% 【第2张图】独占一页 (height=0.95)
\clearpage
\begin{figure}[H]
    \centering
    \includegraphics[width=0.95\textwidth, height=0.95\textheight, keepaspectratio]{vis/fig/Prompt_apx/shot_plan.pdf}
\end{figure}

% =================================================================
% 第三部分：Editor
% =================================================================
\clearpage
\enlargethispage{3cm}

\subsection{Prompt for Editor}

% 【第1张图】与标题在同一页
\begin{figure}[H]
    \centering
    \includegraphics[width=0.95\textwidth, height=0.95\textheight, keepaspectratio]{vis/fig/Prompt_apx/Editor_prompt.pdf}
\end{figure}

% 【第2张图】独占一页
\clearpage
\begin{figure}[H]
    \centering
    \includegraphics[width=0.95\textwidth, height=0.95\textheight, keepaspectratio]{vis/fig/Prompt_apx/FGST.pdf}
\end{figure}

% =================================================================
% 第四部分：Reviewer
% =================================================================
\clearpage
% \enlargethispage{3cm}

\subsection{Prompt for Reviewer}

% 【第1张图】与标题在同一页
\begin{figure}[H]
    \centering
    \includegraphics[width=0.95\textwidth, height=0.95\textheight, keepaspectratio]{vis/fig/Prompt_apx/Check_pro.pdf}
\end{figure}

% 【第2张图】独占一页
\clearpage
\begin{figure}[H]
    \centering
    \includegraphics[width=0.95\textwidth, height=0.95\textheight, keepaspectratio]{vis/fig/Prompt_apx/Check_aes.pdf}
\end{figure}

\clearpage
